# Supplementary material for: Intelligent problem-solving as integrated hierarchical reinforcement learning
Source: arXiv:2208.08731 source file (2022-08-18)
Supplement: Supplementary file 1 [file supplementary.tex]

% \documentclass[fleqn,table]{wlscirep}

% \input{preamble}

% \geometry{left=2cm,%
%                 right=2cm,%
%                 top=2.25cm,%
%                 bottom=2.25cm,%
%                 headheight=12pt,%
%                 headsep=1.45cm,
%                 letterpaper}%
% \fancypagestyle{empty}{
%   \lhead{Preprint, submitted to \textit{Nature Machine Intelligence}}
% }

% \title{Hierarchical principles of embodied reinforcement learning - Supplementary material}

% \author[1,*]{Manfred Eppe}
% \author[2,3]{Christian Gumbsch}
% \author[1]{Matthias Kerzel}
% \author[1]{Phuong D.H. Nguyen}
% \author[2]{Martin V. Butz}
% \author[1]{Stefan Wermter}
% \affil[1]{Universität Hamburg, Germany}
% \affil[2]{Universität Tübingen, Germany}
% \affil[3]{Max Planck Institute for Intelligent Systems, Tübingen, Germany}
% \affil[*]{eppe@informatik.uni-hamburg.de}

% \begin{document}
% \twocolumn

% \flushbottom
% \maketitle

% \thispagestyle{empty}
\onecolumn
\thispagestyle{empty}%
\vskip-36pt%
{\raggedright\sffamily\bfseries\fontsize{20}{25}\selectfont Supplementary information \\[10pt] \Large \newtitle  \par}%
\vskip10pt
{\raggedright\sffamily\fontsize{12}{16}\selectfont  \newauthor \par}

% \vskip25pt%

\begin{infobox}[Glossary]
\label{box:appendix:glossary}

\textbf{Decision-time planning } is a search process over different sequences of potential actions and consequently anticipated changes in the world.
The aim is to determine the best possible sequence of actions and immediate next action to reach a specified goal, to satisfy internal motivational drives, or to maximize a reward or minimize a cost function. 
% , where the agent predicts how the actions change the world. The purpose of decision-time planning is to determine the best possible next action with respect to a specific goal, intention, reward or cost function. 

\noindent \textbf{Background planning} refers to simulating the execution of actions, for the purpose of generating samples for training a behavioural policy. 
In contrast to decision-time planning, background planning does not necessarily happen just-in-time before action execution. It is rather similar to dreaming, in the sense that it simulates action executions to train a behaviour or policy during physically idle times. This reduces the amount of required real-world actions to train a policy, avoids catastrophic forgetting, and fosters selective knowledge consolidation.

\noindent \textbf{Intrinsic motivation}
describes a motivational system that rewards behaviour primarily based on internal goals rather than for some external rewards. 
Here, internal goals refer to all goals that highly depend on subjective, internal representations.
External rewards refer to all rewards found in the environment and are somewhat independent of the subject.
We consider the drive for exploration, curiosity, and playfulness intrinsic motivations. 

% \noindent \textbf{Inference-appropriate state abstraction}
% \noindent \textbf{Inference-fitted state abstraction}
\noindent \textbf{State abstraction}
refers to mapping a lower-level state representation to a higher-level representation.
For instance, high-dimensional raw sensor data are low-level partial state representations, which can be abstracted to high-level discrete symbolic representations\cite{Eppe2019_planning_rl} or low-dimensional continuous vectors produced by convolution and pooling layers in neural networks\cite{Jiang2019_HRL_Language_Abstraction,Lample2018_PlayingFPSGames,Oh2017_Zero-shotTaskGeneralizationDeepRL,Sohn2018_Zero-ShotHRL}.

\noindent \textbf{Action abstraction}
refers to the process of generalizing an action representation. 
For example, the index or label of a context-independent behavioural policy or movement primitive (e.g. \concept{grasp(object)} is an abstract action representation because it points to a much more specific low-level action model, namely the actual policy used to execute the context-specific low-level motor-commands. 

\noindent \textbf{Inference-fitted abstraction} is abstraction such that each representational layer is \emph{appropriate for the level of inference} to be performed on that layer. 
For example, many approaches based on convolutional neural networks are not inference-fitted because the same output of the convolution is passed to all hierarchical RL layers. Therefore, all hierarchical RL layers operate on the same preprocessed state representation, and it is unlikely that the representation is the best fit for all levels of inference.
In contrast, utilizing low-level raw sensor data as appropriate state representations for the low-level reinforcement learning layer and propositional symbolic high-level representations to perform high-level inference  with an action planner is inference-fitted: Here, the low-level control relies on low-level data while the high-level inference performs more effectively with high-level representations, which do not contain all the details of the low-level representation. 

\noindent \textbf{Compositional representations} are data structures that consist of sub-data structures that are subject to semantic rules, which specify how the sub-data structures may be combined. For example, this sentence itself is a data structure that consists of words and grammatical constructions, which are sub-data structures. The sentence is compositional because there exist grammatical rules that are necessary to understand the sentence. Another example for a compositional representation is a disentangled vector representation, where the individual slots of the vector represent individual properties (e.g. angle, colour, rotation or shape of an object). In this case, the semantic rules determine the meaning of each individual slot of the vector.

\noindent \textbf{Mental simulation}
refers to the general ability to anticipate future states of the agent and its environment, where ``states'' can both refer to concrete observations but also to abstract properties of the environment. Note that the temporal reference ``future'' is relative to an assumed starting point in time and independent of the time when the mental simulation is performed. For example, an agent can perform counter-factual mental simulation to anticipate how a past starting state may have had developed differently if the agent had executed a hypothetical course of actions that is different from the actions it actually applied.

\noindent \textbf{Transfer learning}
is a broad term that generally refers to transferring knowledge acquired in a specific context to a new context. 
The term ``transfer'' is partially misleading in the sense that knowledge is usually not transferred between different agents, but rather re-applied in different contexts. Furthermore, transfer learning usually means that learned knowledge is transferred, and not that the transfer is learned. 
In robotic problem-solving, the context is usually a specific problem, and the knowledge is a computational model that provides a solution to it. In RL, the computational model is usually a learned policy, but it can also be a forward model or other data structures. 
For example, consider a policy that has been successfully trained to solve one or more source problems. If the same policy can be re-applied to solve a new unknown target problem the transfer is successful. 
\citet{Perkins1992} propose a distinction between near and far transfer. 
 Near transfer refers to the transfer of skills in similar domains and situations, e.g. using the knowledge from learning to grasp a glass to grasping other objects. Far transfer typically refers to the transfer of solutions between different situations via abstract analogies.

\noindent \textbf{Inductive bias}
refers to a set of assumptions to constrain a learning algorithm. 
% Typically, there are many possible solutions to a problem. With inductive biases, one can incentivize a learning algorithm ``to prioritize one solution (or interpretation) over another'' \cite{Battaglia:2018}. 
% Ideally, inductive biases encode knowledge about the problem and help the algorithm to generalize better to novel data.
Ideally, inductive biases encode general knowledge that is independent of the specific problem so solve, helping the algorithm to generalize better to novel data.
For example, curiosity and other intrinsic motivation models are inductive behavioural biases that potentially improve the data exploration of an agent. 
On the other hand, structural modularizations, convolution, and attention-based information processing, as well as regularization mechanisms are typical inductive learning biases.

\noindent \textbf{Event segmentation}
describes the process of identifying distinct events from a stream of continuous sensorimotor information. Very generally, an event can be any type of segment that is perceived to have a beginning and an end  \cite{Zacks2001_EventStructure}.
Moreover, an event can be typically characterised by distinct interaction dynamics, including particular spatial-relational, force or motor, and entity-respective properties \cite{Butz2016,Butz:2021} (cf. also \autoref{box:appendix:EST}). 

% \noindent \textbf{Epistemic drive}
% refers to the motivational drive of an agent to gain knowledge about itself and its environment. 

\noindent \textbf{Goal-Directed Behaviour}
refers to behaviour, possibly including the direction of attention and thought itself, towards goals. These goals may be activated by motivations, including extrinsic as well as intrinsic motivations, and related epistemic drives.
Goal-directed behaviour thus naturally influences both background planning and decision-time planning, by selectively reflecting on gathered experiences and actively reasoning and planning to solve current tasks respectively

% \noindent \textbf{Zero-shot, one-shot and few-shot problem-solving and learning}
% In machine learning literature, zero-shot learning usually refers to an architecture that can solve a new problem without any new training data.
% One-shot and few-shot learning requires one or only a few new training examples. 
% We adapt this terminology and use the terms zero-shot and few-shot problem-solving to refer to an agent that can solve a new problem without or with only a few any additional training trials. 
 \end{infobox}

% \section{Supplementary information}
% \subsection{Meta survey}
\begin{infobox}[Meta survey of hierarchical reinforcement learning review articles]
\label{box:appendix:meta_RL-survey}
\revv{
At the time of writing this article, we performed a comprehensive meta-search over RL review articles from 2015 to 2020 using the Microsoft Academic search engine, and additional articles from 2021. Our meta-survey yielded the following results: 
The most cited review article on RL since 2015 \citesupp{Arulkumaran2017_DeepRL} dedicates 1/6th of a page out of 16 pages to hierarchical approaches. 
In the second most cited article \citesupp{Garcia2015_safeRLSurvey}, hierarchical RL is not considered at all, i.e, the word stem `hierarchic' does not appear anywhere in the text. 
The third most cited review article \citesupp{Li2018_DeepRL_Overview} dedicates 2/3rd of a page out of 85 total pages to hierarchical RL. 
From 37 RL reviews and surveys published since 2015, only two contain the word stem ``hierarchic'' in their abstract. 
The second edition of the popular RL book by \citet{Sutton:2018} only mentions hierarchies in the twenty-year-old options framework \citesupp{Sutton1999_options} on two pages in the final book chapter and briefly discusses automatic abstraction a few lines later in that chapter. 
Only very recently, \citet{Pateria2021_HRL_Survey} have published a comprehensive survey on HRL.
It appears that researchers continue to struggle with automatically learning RL-suitable hierarchical structures. 
}{E-\ref{rev:editor:form:shorten}}
% \newpage
\end{infobox}

\begin{infobox}[Overview of contemporary hierarchical reinforcement learning approaches]
\label{box:appendix:hrl_review}
% \subsection{Overview of contemporary hierarchical reinforcement learning approaches}
\rev{
In the following, we briefly summarise the results of our comprehensive review of 50 recent (mostly since 2017) hierarchical reinforcement learning methods, as listed in \autoref{tab:hrl_properties}. 

\textbf{Abilities.} 
10 out of 50 reviewed approaches focus on few-shot problem-solving. 
In our article, we reason that planning and transfer learning are the main drivers behind few-shot problem-solving. 
We distinguish here between near and far transfer learning\citesupp{Perkins1992}, where \emph{near} transfer learning denotes transfer between similar contexts and domains between source and target tasks, while \emph{far} transfer considers stronger dissimilarities.
For example, near transfer may simply mean that a robot can grasp a block at a specific location after it has learned to grasp the same block at other locations. 
Near transfer often involves re-using low-level policies \citesupp{Eysenbach2019_DiversityFunction,Frans2018_MetaLearningHierarchies,Heess2016_transferModulControl,Jiang2019_HRL_Language_Abstraction,Li2020_SubPolicy,Qureshi2020_CompAgnosticPol,Sharma2020_DADS,Tessler2017_LifelongHRLMinecraft,Vezhnevets2016_STRAW}.
% Transfer learning may also involve the transfer of other data structures, such as predictive forward models\citesupp{Wu2019_ModelPrimitives}.

% \citet{Vezhnevets2016_STRAW} build on the automatic discovery of transferable macro-actions (plans) to solve problems in discrete 2D-environments, while  \citet{Jiang2019_HRL_Language_Abstraction} use natural language action representations to perform near transfer learning.
% \citet{Qureshi2020_CompAgnosticPol} build on re-usable low-level policies for goal-conditioned hierarchical reinforcement learning. 
% The policies are transferable between similar tasks, e.g. different locomotion tasks with the same agent.

We classify transfer learning between different robot and agent morphologies\citesupp{Devin2017_Transfer_RL,Frans2018_MetaLearningHierarchies,Hejna2020_MorphologicalTransfer} as \emph{far} transfer because the entire sensorimotor apparatus changes, which places the agent in a far dissimilar context.
We identify 11 methods that perform near transfer learning and only four that consider far transfer learning. 
% Far transfer is mostly achieved by transferring high-level skills between different robot morphologies. 

We consider decision-time planning as another method to achieve few-shot problem-solving. 
Our table shows that only eight methods consider decision-time planning, and all of them do this on the high-level layer(s). 

\textbf{Mechanisms.}
All methods perform inference-fitted action abstraction because it is an inherent property of hierarchical reinforcement learning. 
19 methods represent actions in a compositional manner, mostly as subgoals in Cartesian coordinate space. 
Such subgoal-based action representations are not high-level semantic representation in an ontological sense, but they must be called compositional because their individual components (e.g., x, y, and z goal coordinate of an object) constitute a more meaningful representation (a point in 3d space) through clearly defined geometrical rules. 
Only 18 methods perform inference-fitted state abstraction, and for only six methods the abstract state representations can be considered compositional. Note that we do not count state abstractions of visual representations with convolutional neural networks because these are not inference-fitted. 
Intrinsic motivation methods are implemented in 27 of 50 methods, and 22 of them consider intrinsic motivation for achieving subgoals. Only three methods feature curiosity as intrinsic motivation methods, and only six consider diversity. Those that consider diversity are often derived from the options framework and reward the diversity of options. 
Mental simulation is used in only 10 approaches, mostly on the high-level layer(s) only for decision-time planning. There exists only one approach where truly hierarchical mental simulation, i.e., mental simulation on multiple layers, is used\citesupp{Li2017_efficient_learning}. 
Those approaches that feature mental simulation and not decision-time planning perform background planning. 
This is the case for the low-level layers of 2 out of 50 reviewed methods\citesupp{Li2017_efficient_learning,Wu2019_ModelPrimitives}. 

\textbf{Prerequisites.}
Forward models are used in only nine HRL approaches to perform mental simulation for background planning or for decision-time planning. Seven methods do not have an inverse model to select actions for the high-level layer. Instead, they use decision-time planning based on a forward model for the high-level decision-making. One approach performs decision-time planning in the low-level layer \citesupp{Li2017_efficient_learning}. 
}{ E-\ref{rev:editor:form:shorten}; R1-\ref{rev:r1:table_figure}}
\end{infobox}

\begin{infobox}[Example: Compositionality reduces the space of representational mappings]
\label{box:appendix:compositionality-example}
% \subsection{Compositionality reduces the space of representational mappings}
% \label{sec:appendix:compositionality-example}
\revv{
The analogies between two or more  problems in goal-conditioned reinforcement learning are defined by a multidimensional mapping between the initial state space, the goal space, and the action space of these problems. 
For example, given $n_a=4$ action types (e.g. \concept{``grasp'', ``push'', ``move'', ``release''}) and $n_o=4$ compatible object types (e.g. \concept{``glass'', ``cup'', ``tea pot'', ``spoon''}), a non-compositional action-representation requires one distinct symbol for each action-object combination, resulting in $n_o \cdot n_a/2$ possible action mappings. In contrast, an analogy mapping with compositional actions would require searching over possible mappings between action types and, separately, over mappings between objects. Hence, the size of the search space is only $n_o/2 + n_a/2$. 
Thus, compositionality simplifies the identification of analogies because it enables \emph{compositional mappings} between representations. 
}{E-\ref{rev:editor:form:shorten}}
\end{infobox}

\begin{infobox}[From planned behaviour to habits]
\label{box:appendix:automatization}
\revv{
Traditionally, the behaviour of biological agents is divided into two categories: Habitual behaviour or planned behaviour \citesupp{Dolan2013}.
A similar distinction is prevalent in reinforcement learning (RL), where one distinguishes between  model-free and model-based RL: while model-free behaviour is purely learned from reinforcements, in model-based behaviour some form of world model is involved \citesupp{Dolan2013}. 
However,  the continuous learning of action-effect complexes, as proposed by the Theory of Event Coding \citesupp{Hommel2001}, calls the traditional view of a dichotomy between planned and habitual behaviour into question: A particular behaviour seems to become more and more automatised with increasing experience \citesupp{Dayan2009, Dolan2013,ODoherty:2017}. For example, learning to grasp takes time and effort for infants because they must first learn to accurately control their hands and fingers. Later, grasping behaviour happens more or less automatically suggesting that a suitable abstraction of this behaviour has been learned. This implies that planned behaviour and habitual behaviour might be two sides of a continuum \citesupp{Dolan2013} with new behaviour requiring more planning, and thus more computational resources, and habits, on the other side of the spectrum, requiring very little computational resources because they are almost fully automated.}{R2-\ref{rev:r2:habits}, R2-\ref{rev:r2:sugg:automatization}} 

\end{infobox}

\newpage

\begin{infobox}[Event Segmentation Theory]
\label{box:appendix:EST}
There exists a variety of evidence that humans perceive the continuous stream of perceptual information in terms of discrete events \citesupp{Zacks2001_EventStructure}.
According to the Event Segmentation Theory (EST)\citesupp{Zacks2007_EST} these segmentations mirror the internal representation of the unfolding experience.
According to EST, sensorimotor abstractions, or \emph{event models}, provide additional information that can be used for forward predictions\citesupp{Radvansky2011_EventPerception, Zacks2007_EST}. %i.e.~sensorimotor abstractions that encode entities with certain properties and their functional relations in a spatiotemporal framework \citesupp{Radvansky2011_EventPerception}, provide additional information that can be used for forward predictions\citesupp{Zacks2007_EST}.
While observing an event, a specific subset of event models is active until a transient prediction error is registered, resulting in an exchange of the currently active event models  to a new subset that may be better suited for predicting the currently ongoing dynamics\citesupp{Kuperberg:2020tsi, Radvansky2011_EventPerception, Shin:2020tsi, Zacks2007_EST}.
Thus, event models are highly compositional, in the sense that a particular subset of active event models constitutes one particular event.
Furthermore, EST suggests that such prediction error-based segmentations occur on multiple levels of perceptual processing resulting in a hierarchical organisation of event models\citesupp{Zacks2001_EventStructure, Zacks2007_EST}.
EST-inspired computational models demonstrate that such transient forward prediction errors can indeed be used to signal event transitions in video streams or self-explored sensorimotor data in an online fashion
\citesupp{Franklin:2020, Gumbsch2019, Humaidan:2020}.

\end{infobox}

% \cite{Jiang2019_HRL_Language_Abstraction,Lample2018_PlayingFPSGames,Oh2017_Zero-shotTaskGeneralizationDeepRL,Sohn2018_Zero-ShotHRL,Vezhnevets2017_Feudal,Wulfmeier2020_HierachicalCompositionalPolicies,Yang2018_HierarchicalControl}

\begin{table*}[!ht]
{\sffamily 
% The full Excel table is here: \url{https://1drv.ms/x/s!AkFdeL8LlTTlip9lJdytKEfulJ6wdg?e=Fh2nYr}
  \centering
  \captionsetup{singlelinecheck = false, justification = raggedright}
\caption{Abilities, mechanisms and prerequisites of recent hierarchical reinforcement learning  approaches.}
\vspace{-10pt}
  \scriptsize
\rowcolors{2}{TableRowColor}{TableRowColor}
  \begin{tabular}{R{.14\textwidth}  C{.05\textwidth}  C{.06\textwidth}  C{.08\textwidth}  C{.055\textwidth}  C{.055\textwidth}  C{.08\textwidth}  C{.08\textwidth}  C{.08\textwidth}  C{.08\textwidth} }

\arrayrulecolor{black}            
  \rowcolor{TableRowColor}
            & \multicolumn{3}{ c  }{\scshape \large Abilities} & \multicolumn{4}{ c  }{\scshape \large Mechanisms} & \multicolumn{2}{ c }{\scshape \large Prerequisites} \\

\rowcolor{TableRowColor}
  {\scshape \large Approach} & Few-shot problem-solving & Transfer learning --------------- \begin{minipage}{.06\textwidth} N: near \\ F: far \end{minipage} \newline & Decision-time planning ------------------ \begin{minipage}{.08\textwidth} H: high-level \\ L: low-level \end{minipage} \newline &  \multicolumn{2}{ c }
   {
  \begin{minipage}{.13\textwidth} {\centering \vspace{5pt} Sensorimotor abstraction \\ --------------------------- \\} B: basic \\ I: inference-fitted \\ C: compositional \\ \hspace{2pt}  ( actions )~~~~~~~~~ ( states )\end{minipage} 
   } & 
   Intrinsic motivation ------------------- \begin{minipage}{.1\textwidth}C: curiosity \\D: diversity \\SG: subgoals\\[0pt]  \end{minipage} &
   Mental simulation ------------------- \begin{minipage}{.08\textwidth} H: high-level \\ L: low-level \end{minipage} \newline & 
    \newline Forward model -------------------- \begin{minipage}{.08\textwidth} H: high-level \\ L: low-level \end{minipage} \newline & 
   Inverse model / policy ------------------- \begin{minipage}{.08\textwidth} H: high-level \\ L: low-level \end{minipage} \newline \\\hline

\arrayrulecolor{white}

\citetsupp{Akrour2018_RL_StateAbstraction} & - & - & - & I,C & I & - & - & - & H,L\\\hline
\citetsupp{Arulkumaran2016_Classifying_Options_for_Deep_RL} & - & - & - & I & - & - & - & - & H,L\\\hline
\citetsupp{Bacon2017_OptionCritic} & - & - & - & I & - & - & - & - & H,L\\\hline
\citetsupp{barreto2020fast} & (X) & F & - & I & - & - & - & - & H,L\\\hline
\citetsupp{Beyret2019_DotToDot} & - & - & - & C & - & - & - & - & H,L\\\hline
\citetsupp{Blaes2019_CWYC} & - & - & H & I & - & C, SG & H & H,L & L\\\hline
\citetsupp{Chuck2020_HyPe} & - & - & - & I & - & C & - & - & H,L\\\hline
\citetsupp{Dietterich2000_StateAbstraction_MAXQ} & - & - & - & I & I,C & SG & - & - & H,L\\\hline
\citetsupp{Eppe2019_planning_rl} & - & - & H & I,C & I,C & SG & H & H & L\\\hline
\citetsupp{Eysenbach2019_DiversityFunction} & - & N & - & I & - & D & - & - & H,L\\\hline
\citetsupp{Frans2018_MetaLearningHierarchies} & (X) & F & - & I & - & - & - & - & H,L\\\hline
\citetsupp{Ghazanfari2020_AssociationRules} & - & - & - & I & I & - & - & - & H,L\\\hline
\citetsupp{Ghosh2019_ActionableRep} & - & - & - & I & I & SG & - & - & H,L\\\hline
\citetsupp{Haarnoja2018_LatentSpacePoliciesHRL} & - & - & - & I & - & SG & - & - & H,L\\\hline
% \citetsupp{Hafez2020_dual-system} &  &  &  &  &  &  &  &  & \\\hline
\citetsupp{Han2020_hierarchicalSelfOrga} & X & N & - & I & - & - & - & - & H,L\\\hline
\citetsupp{Heess2016_transferModulControl} & X & F & - & I & - & - & - & - & H,L\\\hline
\citetsupp{Hejna2020_MorphologicalTransfer} & X & F & - & C & - & - & - & - & H,L\\\hline
\citetsupp{jaderberg2019human} & - & N & - & I & I & SG,(D) & - & - & H,L\\\hline
\citetsupp{Jiang2019_HRL_Language_Abstraction}  & X & N & - & I,C & B & - & - & - & H,L\\\hline
\citetsupp{Kulkarni2016_HDQN} & - & - & - & I & I,C & SG & - & - & H,L\\\hline
\citetsupp{Levy2019_Hierarchical} & - & - & - & C & - & SG & - & - & H,L\\\hline
\citetsupp{Li2017_efficient_learning} & - & - & H & I,C & - & - & H,L & H,L & H,L\\\hline
\citetsupp{Li2020_SubPolicy} & X & N & - & I & - & - & - & - & H,L\\\hline
\citetsupp{Lyu2019_SDRL} & - & - & H & I & I,C & SG & H & H & L\\\hline
\citetsupp{Ma2020_MultiAgentHRL} & - & - & H & I & I & - & H & H & L\\\hline
\citetsupp{Machado2017_PVF_Laplace_OptionDiscovery} & - & - & - & I & I & D & - & - & H,L\\\hline
\citetsupp{Nachum2018_HIRO} & - & - & - & C & - & SG & - & - & H,L\\\hline
\citetsupp{Oh2017_Zero-shotTaskGeneralizationDeepRL} & X & N & - & I,C & I & SG & - & - & H,L\\\hline
\citetsupp{Qiao_2020_HRL-Driving} & - & - & - & I & - & SG & - & - & H,L\\\hline
\citetsupp{Qureshi2020_CompAgnosticPol}	& -	& F& 	-& 	I,C	&-& 	SG,D& 	-& 	-& 	H,L \\\hline
\citetsupp{Rafati2019_model-free_rep_learning} & - & - & - & C & - & SG & - & - & H,L\\\hline
\citetsupp{Rasmussen2017_NeuralHRL} & - & N & - & I,(C) & I & SG & - & - & H,L\\\hline
\citetsupp{Riedmiller2018_SAC-X} & - & - & - & I & - & SG & - & - & H,L\\\hline
\citetsupp{Roeder2020_CHAC} & - & - & - & C & - & C,SG & - & - & H,L\\\hline
\citetsupp{Saxe2017_HRL_Multitask_LMDP} & - & - & - & I,C & - & SG & - & - & H,L\\\hline
\citetsupp{Schaul2013_Better_Generalization_with_Forecasts} & - & - & - & I & I,C & - & - & - & H,L\\\hline
\citetsupp{Shankar2020_MotorPrimitives} & - & - & - & I & - & D & - & - & H,L\\\hline
\citetsupp{Sharma2020_DADS} & X & N & H & I & - & D & H & H & L\\\hline
\citetsupp{silver2016mastering} & - & - & H & I & I & - & H & H & L\\\hline
\citetsupp{Sohn2018_Zero-ShotHRL} & X & N & - & I,C & I & SG & - & - & H,L\\\hline
\citetsupp{sutton2011horde} & - & (N) & - & - & I & - & L & L & L\\\hline
\citetsupp{Tessler2017_LifelongHRLMinecraft} & (X) & N & - & I,C & - & - & - & - & H,L\\\hline
\citetsupp{Vezhnevets2017_Feudal} & - & - & - & I & I & - & - & - & H,L\\\hline
\citetsupp{Vezhnevets2020_OPRE} & - & - & - & I,C & I,C & -  & - & - & H,L\\\hline
\citetsupp{Wu2019_ModelPrimitives}	& -	& N	& -	& I	& -	& -	& L	& L	& H,L \\\hline
\citetsupp{Wulfmeier2020_HierachicalCompositionalPolicies} & - & N & - & I & - & - & - & - & H,L\\\hline
\citetsupp{Yamamoto2018_RL_Planning} & - & - & H & I,C & - & SG & H & H & L\\\hline
\citetsupp{Yang2018_PEORL} & - & - & H & I & - & SG & H & H & L\\\hline
\citetsupp{Yang2018_HierarchicalControl} & - & - & - & I & - & - & - & - & H,L\\\hline
\citetsupp{Zhang2020_AdjancentSubgoals} & - & - & - & C & - & SG & - & - & H,L\\\hline
  \end{tabular}
 \normalsize
    \label{tab:hrl_properties}
}
\end{table*}

\newpage

% \input{bibliography}

% \addtolength{\textheight}{-2.5cm}

% \input{appendix}

% \end{document}
