# Supplementary material for: Intelligent problem-solving as integrated hierarchical reinforcement learning
Source: arXiv:2208.08731 source file (2022-08-18)
Supplement: Supplementary file 3 [file appendix.tex]

\appendix
\section{A Brief Meta-Survey on Reinforcement Learning}
\label{sec:appendix:meta_RL-survey}
To analyze how deeply the hierarchical aspects in reinfocement learning are currently investigated, we perform the following meta-survey. 

We use the Microsoft Academic search API \cite{} to access the Microsoft Academic Graph database with over 200,000 research papers. The following results have been obtained with a snapshot of the database taken on March, 20th, 2020. 

We search for articles assigned to the category ``reinforcement learning'' with more than five citations and published between 2015 and 2020. From the resulting XXXX articles, we select those that contain the words ``reinforcement'' and one of the words ``survey'', ``review'' or ``overview'' in the title. The resulting list contains 37 articles. From these articles only 2 contain the word stem ``hierarchic'' in the abstract.
